# Supplementary material for: The fundamental drivers of electrochemical barriers
Source: arXiv:2306.05521 ancillary file (2023-11-08)
Supplement: Supplementary file 1 [file SupportingInformation.pdf]

# The fundamental drivers of electrochemical barriers

Xi Chen[1], Georg Kastlunger[2], and Andrew A. Peterson[3]

[1]*School of Engineering, Brown University, Providence, Rhode Island, 02912, USA*
[2]*Department of Physics, Technical University of Denmark, DK-2800, Kongens Lyngby, Denmark*
[3]*School of Engineering, Brown University, Providence, Rhode Island, 02912, USA*

## Contents

**1 Curved scaling model** **2**

**2 Thermodynamics of energy change with potential** **5**

**3 Full barrier calculation results** **7**

**4 Work function and excess electrons** **10**

**5 Grand-canonical electronic structure calculations** **11**

**6 Python class to fit scaling model** **12**

**7 References** **15**

# 1 Curved scaling model

In earlier work [1,2], we introduced a simple formalism to capture the limiting behavior of reactions as they become strongly downhill and strongly uphill. This equation relates the transition state energy $E^\ddagger$ to the reaction energy $\Delta E$, using a single parameter $b$ (which can be interpreted as the barrier when $\Delta E = 0$):

$$E^\ddagger = \frac{(\Delta E + 4b)^2}{16b}$$

which is valid in the domain $-4b \leq \Delta E \leq +4b$; outside of this range $E^\ddagger$ takes on limiting values of 0 when $\Delta E \ll 0$ and $\Delta E$ when $\Delta E \gg 0$. We note that although this bears a superficial resemblance to Marcus theory, it is is only intended to capture the limiting behavior implied by the Hammond–Leffler postulate, and can be expect to apply to general reactions which have a variable driving force (that is, not solely or specifically electron-transfer reactions). We would expect a relatively noiseless fit to this form for functions with a continuously variable driving force—like potential in the current work, or other works focusing on strain [3,4] or electrostatic catalysis [5]—while we'd expect a noisier fit when the driving force changes as a result of a substitution effect, such as trends among catalyst surfaces [6, 7] or organic functional groups [8].

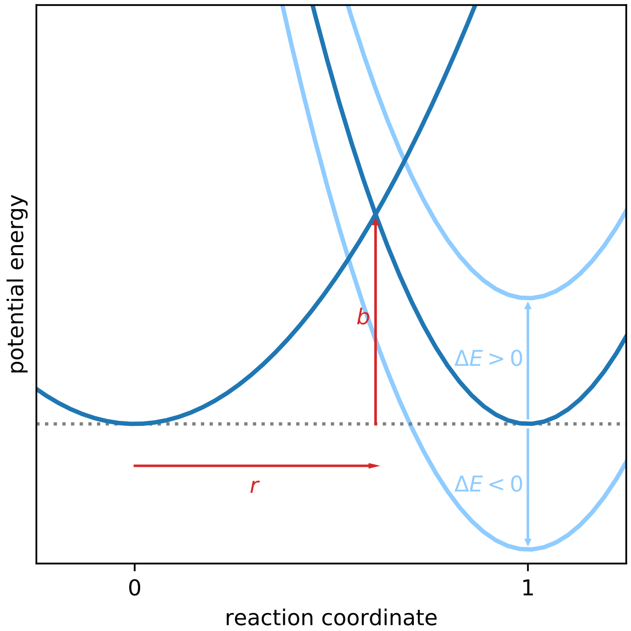


**Figure S1:** The intersection between uneven parabolas captures the limiting behavior of the functional relationship between reaction barriers and reaction energetics. $b$ is the barrier height when $\Delta E = 0$, and $0 \leq r \leq 1$ is the skew parameter.

Here, we introduce a second parameter to this model to allow for skew in the relationship. The parameter $b$ retains its previous meaning, while the second parameter $r$ indicates the skew, as shown schematically in Figure S1. This model is based on the point of intersection of parabolas of unequal width; $r$ indicates the relative position of the point of intersection (when at equal energy, $\Delta E = 0$). Thus, when $r = \frac{1}{2}$, the previous one-parameter (symmetric) model is recovered; when $r < \frac{1}{2}$ the

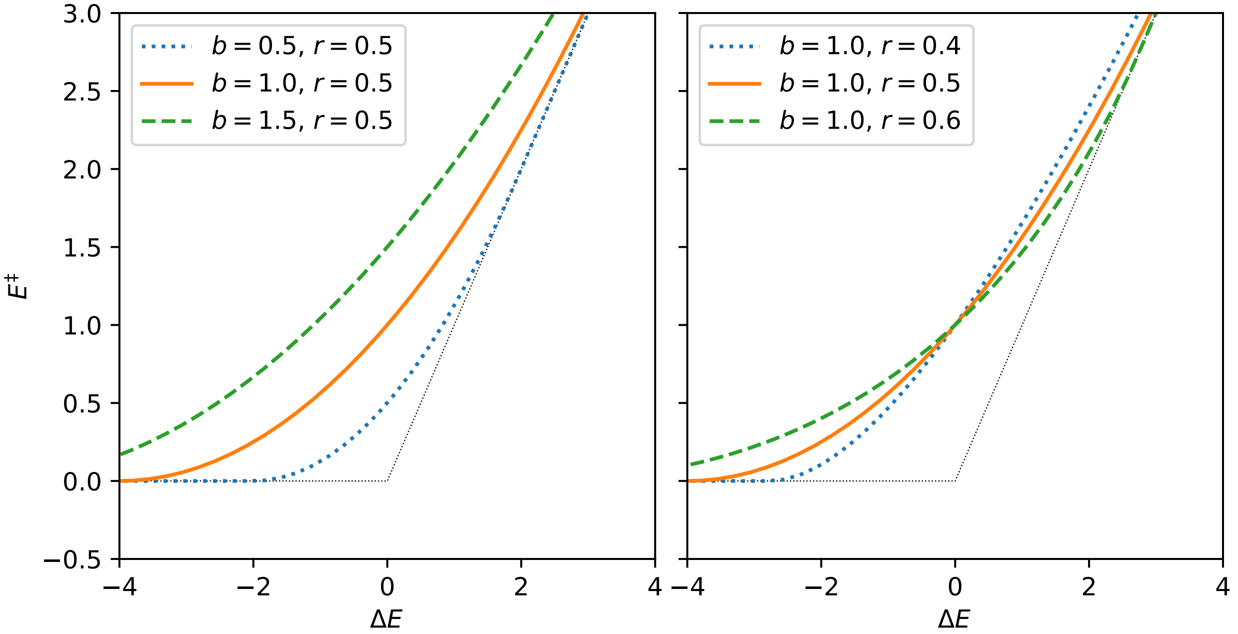


**Figure S2:** Example of scaling relations with various parameter values of $b$ and $r$.

left parabola is narrower, and vice versa for $r > \frac{1}{2}$. In Figure S2 we show the effect of changing $b$ and $r$ independently.

While having only two parameters, the functional form of this relationship is more elaborate:

$$E^{\ddagger} = b \left[ \frac{(1-r)\sqrt{1 - \frac{\Delta E}{b}(2r-1)} - r}{2r-1} \right]^2 \tag{1}$$

which is valid in the domain

$$\frac{-1}{(r-1)^2} < \frac{\Delta E}{b} < \frac{1}{r^2}$$

and outside this range it takes on the same limiting values as the one-parameter model; it continuously approaches these limits. Like a traditional linear scaling relation, this model has only two parameters, yet unlike the linear model, it correctly approaches the limiting behavior and captures the inherent curvature of transition-state scaling. While the equation is certainly more complicated than that of a line, it is straightforward to find best-fit values of $b$ and $r$ using any modern scientific package. We provide a simple python class that accomplishes this at the end of this document.

## Derivation outline

We briefly provide the derivation of equation (1), using Figure S1 as a guide, taking $x$ and $y$ to be the abscissa and ordinate, respectively. The equations of the left and right parabolas are:

$$y_{\mathrm{L}} = b\frac{x^2}{r^2}$$

$$y_{\mathrm{R}} = b\frac{(x-1)^2}{(r-1)^2} + \Delta E$$

$E^{\ddagger}$ is the value of $y_{\mathrm{L}}$ (or $y_{\mathrm{R}}$) at the point of intersection $x^*$, which is found by setting $y_{\mathrm{L}} = y_{\mathrm{R}}$ and solving for $x$, in the domain $0 < x < 1$. After algebraic manipulation, and keeping only the negative root, the point of intersection $x^*$ is:

$$x^* = r \cdot \frac{r - \sqrt{r^2 - (2r-1)\left(1 + \frac{\Delta E}{b}\,(r-1)^2\right)}}{2r-1}$$

Since $E^{\ddagger} = y_{\mathrm{L}}(x^*)$, plugging this result in to $y_{\mathrm{L}}$ leads to equation (1), upon re-arrangement.

# 2 Thermodynamics of energy change with potential

At constant potential, calculations take place in the electronically grand-canonical ensemble. The grand-potential energy is defined as $\Phi \equiv A - \mu N$, where $A$ is the Helmholtz free energy, $\mu$ is the chemical potential of electrons in the system, and $N$ is the number of electrons, which for convenience we define to be the excess electrons (beyond charge neutrality). See, for example, Lindgren *et al.* [2] for details and the distinction between grand-potential and grand-canonical energies. The fundamental equations for $A$ and $\Phi$ are

$$dA = -SdT + PdV + \sum_i F_i dx_i + \mu\, dN$$

$$d\Phi = -SdT + PdV + \sum_i F_i dx_i - N d\mu$$

The symbols above take on their usual thermodynamic meanings: $S$ is entropy, $T$ is electronic temperature, $P$ is pressure, $V$ is volume, $F_i$ is a force component on an atom, and $x_i$ is an atomic position component. We are interested in how this energy ($\Phi$) changes with potential. In this ensemble, it will be most natural to evaluate the derivative at constant $T, V, \{\vec{x}_i\}$; for brevity,[1] we'll only denote $\{\vec{x}_i\}$ in the following. Using standard thermodynamic manipulations, we can simplify the partial derivative:

$$\left(\frac{\partial \Phi}{\partial \phi}\right)_{\{\vec{x}_i\}} = \left(\frac{\partial\left[A - \mu N\right]}{\partial \phi}\right)_{\{\vec{x}_i\}}$$

$$\left(\frac{\partial \Phi}{\partial \phi}\right)_{\{\vec{x}_i\}} = \left(\frac{\partial A}{\partial \phi}\right)_{\{\vec{x}_i\}} - \mu\left(\frac{\partial N}{\partial \phi}\right)_{\{\vec{x}_i\}} - N\left(\frac{\partial \mu}{\partial \phi}\right)_{\{\vec{x}_i\}}$$

$$\left(\frac{\partial \Phi}{\partial \phi}\right)_{\{\vec{x}_i\}} = \left(\frac{\partial A}{\partial N}\right)_{\{\vec{x}_i\}}\left(\frac{\partial N}{\partial \phi}\right)_{\{\vec{x}_i\}} - \mu\left(\frac{\partial N}{\partial \phi}\right)_{\{\vec{x}_i\}} - N\left(\frac{\partial \mu}{\partial \phi}\right)_{\{\vec{x}_i\}}$$

$$\left(\frac{\partial \Phi}{\partial \phi}\right)_{\{\vec{x}_i\}} = \mu\left(\frac{\partial N}{\partial \phi}\right)_{\{\vec{x}_i\}} - \mu\left(\frac{\partial N}{\partial \phi}\right)_{\{\vec{x}_i\}} - N\left(\frac{\partial \mu}{\partial \phi}\right)_{\{\vec{x}_i\}}$$

$$\left(\frac{\partial \Phi}{\partial \phi}\right)_{\{\vec{x}_i\}} = -N\left(\frac{\partial \mu}{\partial \phi}\right)_{\{\vec{x}_i\}}$$

Since the chemical potential of an electron changes with potential as $\mu = \mu^0 - e\phi$ (where $e$ is the positive electronic charge constant and $\mu^0$ is the electron's chemical potential at 0 V), then $\left(\frac{\partial \mu}{\partial \phi}\right)_{\{\vec{x}_i\}} = -e\left(\frac{\partial \phi}{\partial \phi}\right)_{\{\vec{x}_i\}} = -e$, leaving

$$\boxed{\left(\frac{\partial \Phi}{\partial \phi}\right)_{\{\vec{x}_i\}} = eN}$$

[1] Note that since the nuclei have fixed position in any image, the temperature here refers to the electronic temperature, which is non-zero. See Lindgren [2] and references therein for full details. The $T$ and $V$ subscripts will be unimportant in the current analysis, but are noted for rigor.

This expression is exact; it did not rely on a truncated Taylor expansion or assumption of a capacitor model. Note that this form does not imply a linear relation between energy and potential: rather, because $N$ typically changes linearly with potential, this is consistent with the well-known parabolic relation.

**Change in energy between two images.** Therefore, to evaluate the change in energy between two fixed atomic configurations A and B, we simply have

$$\left(\frac{\partial\left(\Phi_{\mathrm{B}}-\Phi_{\mathrm{A}}\right)}{\partial\phi}\right)_{\{\vec{x}_i\}_{\mathrm{A}},\{\vec{x}_i\}_{\mathrm{B}}}=\left(\frac{\partial\Phi_{\mathrm{B}}}{\partial\phi}\right)_{\{\vec{x}_i\}_{\mathrm{B}}}-\left(\frac{\partial\Phi_{\mathrm{A}}}{\partial\phi}\right)_{\{\vec{x}_i\}_{\mathrm{A}}}$$

$$=e\left(N_{\mathrm{B}}-N_{\mathrm{A}}\right)$$

If we assign B to be the transition state and A to be the pseudo-initial state, we recover the equation presented in the main text:

$$\boxed{\left(\frac{\partial E^{\ddagger}}{\partial\phi}\right)_{\{\vec{x}_i\}}=eN^{\ddagger}}$$

# 3 Full barrier calculation results

The full set of converged reaction pathways are shown in Figures S3 and S4.

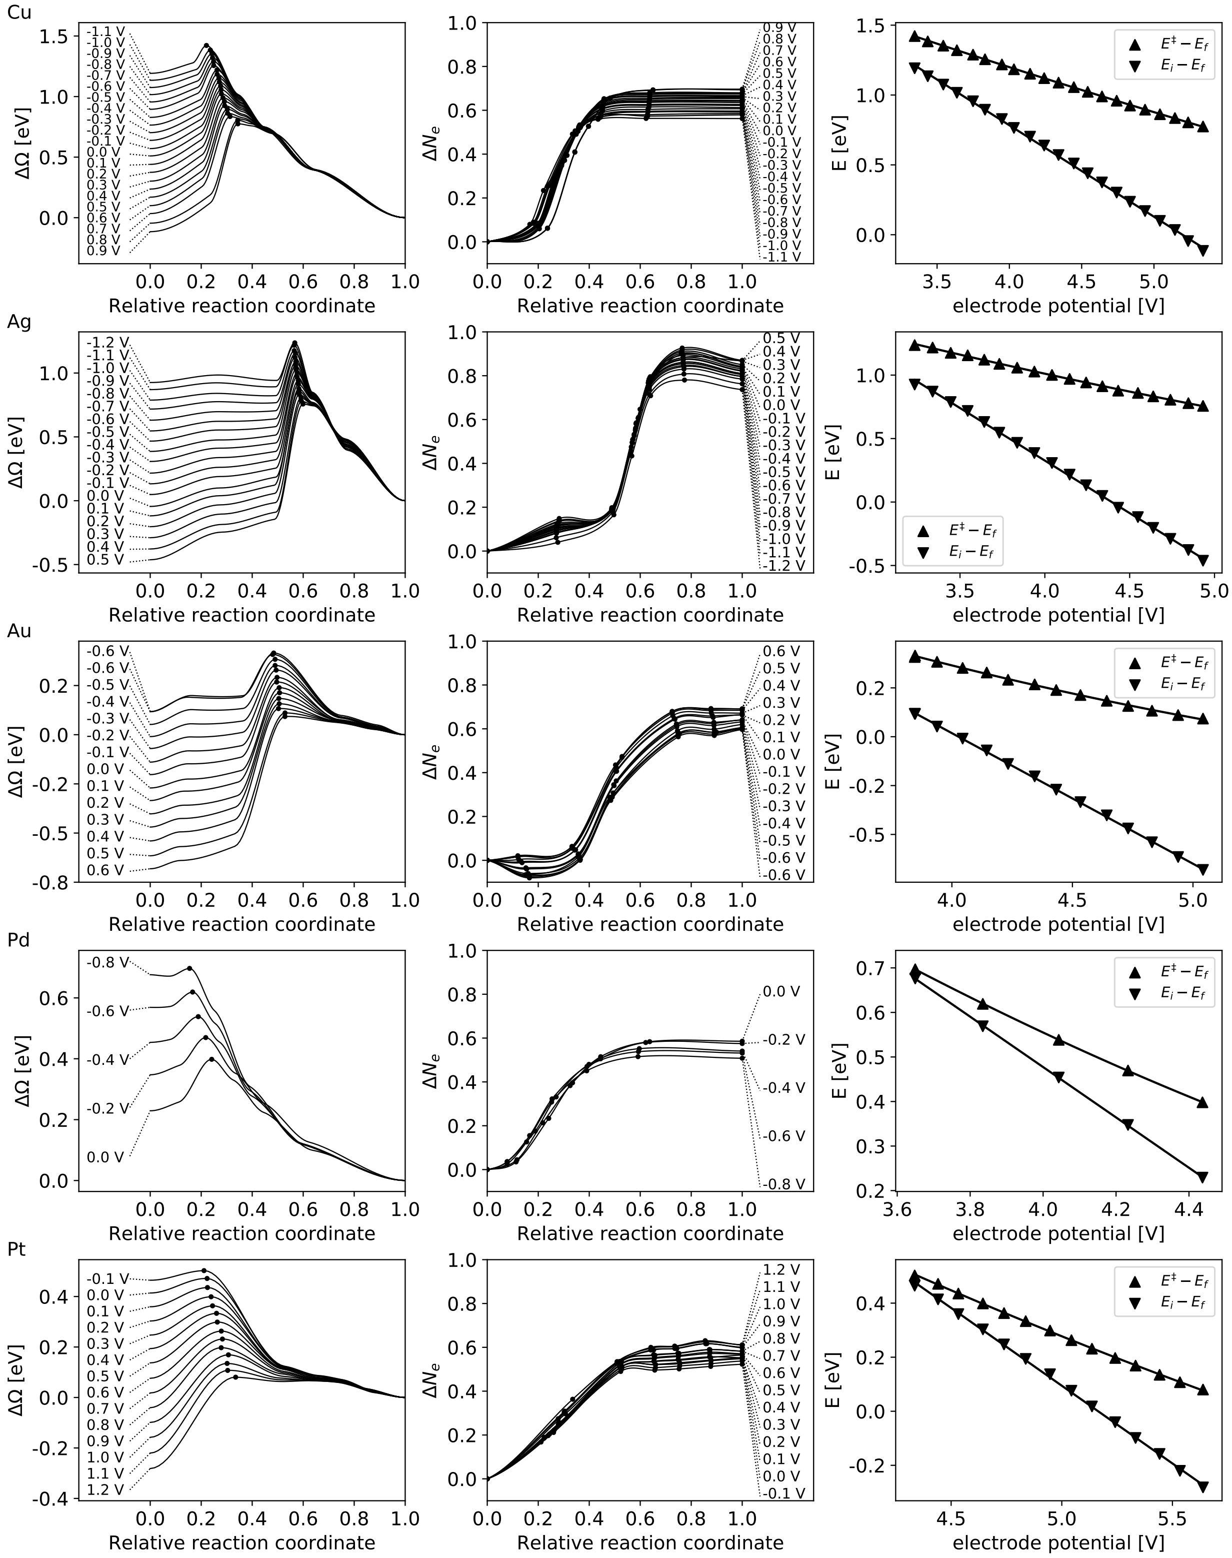


**Figure S3:** Full set of barrier and charge-transfer calculations. Each point represents a converged DyNEB calculation at a fixed potential. (Continued on Figure S4.)

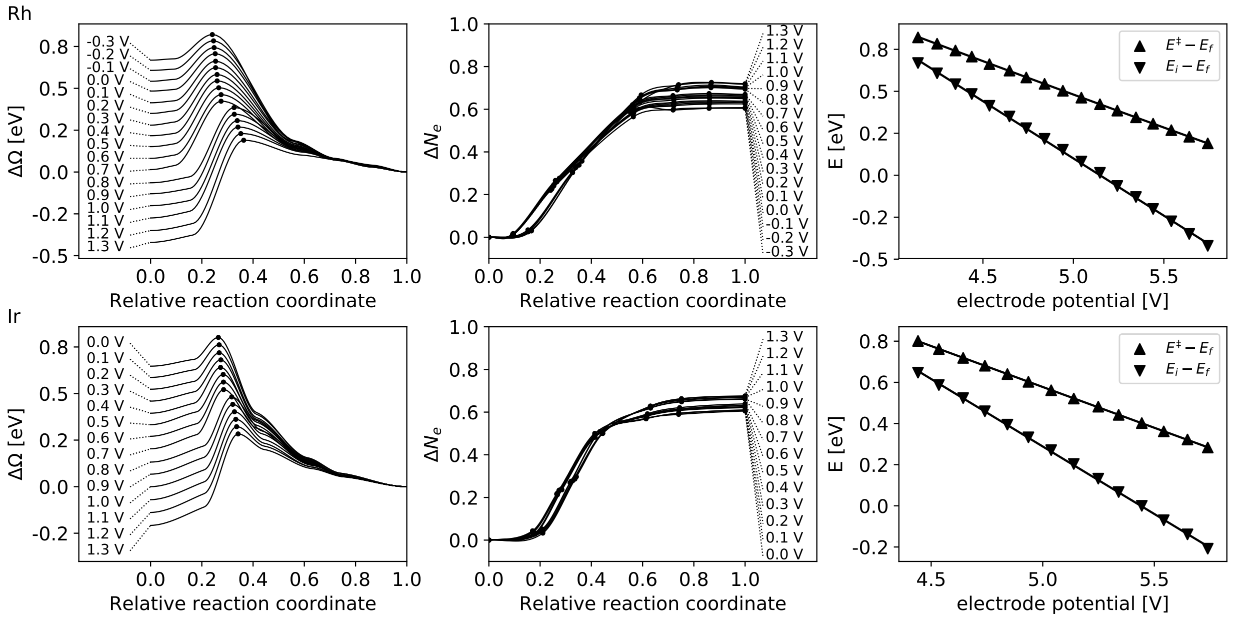


**Figure S4:** Full set of barrier and charge-transfer calculations. Each point represents a converged DyNEB calculation at a fixed potential. (Continued from Figure S3.)

# 4 Work function and excess electrons

As mentioned in the main text, the number of electrons that a potentiostat—whether physical or computational—needs to supply to a surface in order to reach 0 $V_{SHE}$ is, to first order, a function of that material's work function. We show this to be the case for the current work in Figure S5, which compares the (polycrystalline) work function as reported by Michaelson in 1977 [9] to the number of electrons required by SJM reach 0 $V_{SHE}$. This shows an excellent correlation. We note that the potential of zero-charge should also make an excellent descriptor for this quantity; our choice to use work function was to use the simpler quantity.

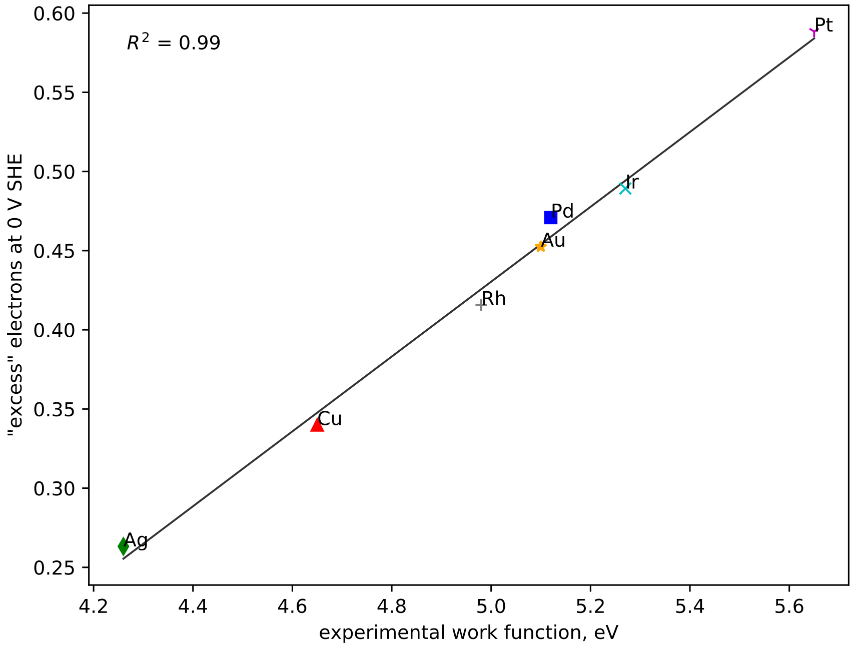


**Figure S5:** Relationship between experimentally tabulated work function [9] and the amount of excess electrons needed by the Solvated Jellium method (SJM) to reach 0 $V_{SHE}$.

# 5 Grand-canonical electronic structure calculations

The solvated jellium (SJ) method [10] was used to perform constant-potential electronic structure calculations, in the electronically grand-canonical ensemble [2]. This method automatically holds the electrode potential at a specified value by manipulating the number of electrons in the simulation, in a manner that allows reaction barriers to be readily calculated at a range of potentials. The SJ method was used as implemented in the electronic structure code GPAW [11, 12]. A Monkhorst–Pack $k$-point grid of $4 \times 4 \times 1$ was employed and BEEF-vdW [13] was used as the exchange–correlation functional. Initial and final structures were relaxed until the maximum force was below 0.03 eV/Å and saddle points were converged to 0.05 eV/Å.

Seven metal surfaces—Cu, Ag, Au, Pd, Pt, Rh, and Ir—consisting of spin-paired late-transition metals were chosen to elucidate trends in this study. All surfaces were structured in the face-centered cubic (fcc) crystal structure with the (111) facet exposed and with an explicit water layer in a hexagonal, ice-like structure. The water layer can exist in an H-down or H-up geometry, depending upon the specific metal surface and potential [14, 15], and reaction pathways can expect to differ between the two configurations. Under most conditions studied here, the H-down structures are stable, and we adopt this geometry for all systems reported here in order to make clean comparisons between systems. For all metals except Cu and Ag, the final state was taken to be an ontop site; for Cu and Ag, this relaxed to the fcc site at certain potentials, therefore the final state was taken as fcc for these two metals. This choice of binding sites causes relative binding strengths across materials to differ from published studies that adopt a uniform binding site. The reaction barriers were calculated in an accelerated manner with the DyNEB approach [16]. All simulations were interfaced via the Atomic Simulation Environment (ASE) [17, 18]

# 6 Python class to fit scaling model

It is straightforward to use nonlinear regression from any numerical package to fit equation (1) to a set of barrier data. For convenience, we provide python code used in our group for this purpose below. (Tested against scipy version 1.8.0 and numpy version 1.21.5.) This code lives in our group's publicly available software repository[2], a newer version may be available there.

File attached here.

```python
import numpy as np
from scipy.optimize import minimize


class DoubleParabola:

    def __init__(self, deltaEs=None, barriers=None, no_parameters=2,
                 b=None, r=None):
        """
        You have two options:
        (1) Initialize with matched lists of energy change of the reaction
        and reaction barriers, and the number of parameters (1 or 2) for the
        model. Will try to fit the model immediately.
        (2) Initialize with the parameters directly; that is supply
        b or (b and r).
        """
        self.parameters = {}
        if b is not None:
            # Must be initializing directly.
            self.parameters['b'] = b
            if r is not None:
                self.parameters['r'] = r
                self._no_parameters = 2
            else:
                self._no_parameters = 1
        else:
            self._deltaEs = deltaEs
            self._barriers = barriers
            self._no_parameters = no_parameters
            self.fit()

    def fit(self, bguess=None, rguess=None):
        if bguess is None:
            # Fitting can be sensitive to initial guess, so
            # estimate b (barrier at deltaE=0) from linear fit.
            # It's equivalent to the intercept.
            bguess = np.polyfit(self._deltaEs, self._barriers, deg=1)[1]
        if rguess is None:
            rguess = 0.49
        if self._no_parameters not in [2]:
            raise NotImplementedError()
        ans = minimize(self._get_loss, x0=[bguess, rguess])
        self.parameters['b'] = ans.x[0]
        self.parameters['r'] = ans.x[1]
```

[2]Currently at `https://bitbucket.org/andrewpeterson/pgroup`

```python

    def _get_loss(self, x):
        """Loss function for use with scipy minimize."""
        if self._no_parameters == 2:
            b, r = x
        elif self._no_parameters == 1:
            b = x[0]
            r = None
        loss = 0.
        for deltaE, barrier in zip(self._deltaEs, self._barriers):
            predicted_barrier = self.get_barrier(deltaE, b, r)
            loss += (predicted_barrier - barrier)**2
        return loss

    def get_edges(self, b=None, r=None):
        """Returns the edges of the curved region."""
        if self._no_parameters == 1:
            b = self.parameters['b'] if b is None else b
            return -4. * b, 4. * b
        b = self.parameters['b'] if b is None else b
        r = self.parameters['r'] if r is None else r
        lower = - b / (1. - r)**2
        upper = b / r**2
        return lower, upper

    def get_barrier(self, deltaE, b=None, r=None):
        """Returns the predicted barrier for a given deltaE value.
        Defaults to using fit b (and r) value, but they can optionally
        be supplied. Note if only b is supplied, a one-parameter model
        is assumed.
        """
        no_parameters = None
        if (b is not None) and (r is None):
            no_parameters = 1
        if (b is not None) and (r is not None):
            no_parameters = 2
        if no_parameters is None:
            no_parameters = self._no_parameters
        if b is None:
            b = self.parameters['b']
        if (r is None) and (no_parameters == 2):
            r = self.parameters['r']
        lower, upper = self.get_edges(b, r)
        if deltaE < lower:
            return 0.
        elif deltaE > upper:
            return deltaE
        if no_parameters == 1:
            return (deltaE + 4. * b)**2 / (16. * b)
        else:
            if r == 0.5:
                return self.get_barrier(deltaE, b)
            ans = (1. - r)
            ans *= np.sqrt(1. - deltaE / b * (2. * r - 1.))
```

```
            ans -= r
            ans /= 2. * r - 1.
            ans *= ans
            ans *= b
            return ans

    def __call__(self, deltaE, b=None, r=None):
        """Returns the predicted barrier."""
        return self.get_barrier(deltaE, b, r)
```

# 7 References

[1] Lindgren, P.; Kastlunger, G.; Peterson, A.A. A Challenge to the $G{\sim}0$ Interpretation of Hydrogen Evolution. *ACS Catal.* **2020**; 10, 121–128.

[2] Lindgren, P.; Kastlunger, G.; Peterson, A.A. Electrochemistry from the atomic scale, in the electronically grand-canonical ensemble. *The Journal of Chemical Physics* **2022**; 157, 180902.

[3] Khorshidi, A.; Violet, J.; Hashemi, J.; Peterson, A.A. How strain can break the scaling relations of catalysis. *Nature Catalysis* **2018**; 1, 263–268.

[4] Zeng, C.; Maark, T.A.; Peterson, A.A. Strain in Catalysis: Rationalizing Material, Adsorbate, and Site Susceptibilities to Biaxial Lattice Strain. *The Journal of Physical Chemistry C* **2022**; 126, 20892–20902.

[5] Hoffmann, N.M.; Wang, X.; Berkelbach, T.C. Linear Free Energy Relationships in Electrostatic Catalysis. *ACS Catalysis* **2022**; 12, 8237–8241.

[6] Wang, S.; Petzold, V.; Tripkovic, V.; Kleis, J.; Howalt, J.G.; Skúlason, E.; Fernández, E.M.; Hvolbæk, B.; Jones, G.; Toftelund, A.; Falsig, H.; Björketun, M.; Studt, F.; Abild-Pedersen, F.; Rossmeisl, J.; Nørskov, J.K.; Bligaard, T. Universal transition state scaling relations for (de)hydrogenation over transition metals. *Phys. Chem. Chem. Phys.* **2011**; 13, 20760–20765.

[7] Wang, S.; Temel, B.; Shen, J.; Jones, G.; Grabow, L.C.; Studt, F.; Bligaard, T.; Abild-Pedersen, F.; Christensen, C.H.; Nørskov, J.K. Universal Brønsted–Evans–Polanyi Relations for C–C, C–O, C–N, N–O, N–N, and O–O Dissociation Reactions. *Catalysis Letters* **2011**; 141, 370–373.

[8] Evans, M.G.; Polanyi, M. Inertia and driving force of chemical reactions. *Trans. Faraday Soc.* **1938**; 34, 11–24.

[9] Michaelson, H.B. The work function of the elements and its periodicity. *Journal of Applied Physics* **1977**; 48, 4729–4733.

[10] Kastlunger, G.; Lindgren, P.; Peterson, A.A. Controlled-Potential Simulation of Elementary Electrochemical Reactions: Proton Discharge on Metal Surfaces. *The Journal of Physical Chemistry C* **2018**; 122, 12771–12781.

[11] Mortensen, J.J.; Hansen, L.B.; Jacobsen, K.W. Real-space grid implementation of the projector augmented wave method. *Phys. Rev. B* **2005**; 71, 035109.

[12] Enkovaara, J.; Rostgaard, C.; Mortensen, J.J.; Chen, J.; Dułak, M.; Ferrighi, L.; Gavnholt, J.; Glinsvad, C.; Haikola, V.; Hansen, H.A.; Kristoffersen, H.H.; Kuisma, M.; Larsen, A.H.; Lehtovaara, L.; Ljungberg, M.; Lopez-Acevedo, O.; Moses, P.G.; Ojanen, J.; Olsen, T.; Petzold, V.; Romero, N.A.; Stausholm-Møller, J.; Strange, M.; Tritsaris, G.A.; Vanin, M.; Walter, M.; Hammer, B.; Häkkinen, H.; Madsen, G.K.H.; Nieminen, R.M.; Nørskov, J.K.; Puska, M.; Rantala, T.T.; Schiøtz, J.; Thygesen, K.S.; Jacobsen, K.W. Electronic structure calculations

with GPAW: a real-space implementation of the projector augmented-wave method. *J. Phys.: Condens. Matter* **2010**; 22, 253202.

[13] Larsen, A.H.; Kuisma, M.; Löfgren, J.; Pouillon, Y.; Erhart, P.; Hyldgaard, P. libvdwxc: a library for exchange–correlation functionals in the vdW-DF family. *Modelling and Simulation in Materials Science and Engineering* **2017**; 25, 065004.

[14] Schnur, S.; Groß, A. Properties of metal–water interfaces studied from first principles. *New Journal of Physics* **2009**; 11, 125003.

[15] Sakong, S.; Forster-Tonigold, K.; Groß, A. The structure of water at a Pt(111) electrode and the potential of zero charge studied from first principles. *The Journal of Chemical Physics* **2016**; 144, 194701.

[16] Lindgren, P.; Kastlunger, G.; Peterson, A.A. Scaled and dynamic optimizations of Nudged Elastic Bands. *Journal of Chemical Theory and Computation* **2019**; 15, 5787–5793.

[17] Larsen, A.H.; Mortensen, J.J.; Blomqvist, J.; Castelli, I.E.; Christensen, R.; Dułak, M.; Friis, J.; Groves, M.N.; Hammer, B.; Hargus, C.; Hermes, E.D.; Jennings, P.C.; Jensen, P.B.; Kermode, J.; Kitchin, J.R.; Kolsbjerg, E.L.; Kubal, J.; Kaasbjerg, K.; Lysgaard, S.; Maronsson, J.B.; Maxson, T.; Olsen, T.; Pastewka, L.; Peterson, A.; Rostgaard, C.; Schiøtz, J.; Schütt, O.; Strange, M.; Thygesen, K.S.; Vegge, T.; Vilhelmsen, L.; Walter, M.; Zeng, Z.; Jacobsen, K.W. The atomic simulation environment—a Python library for working with atoms. *Journal of Physics: Condensed Matter* **2017**; 29, 273002.

[18] Bahn, S.R.; Jacobsen, K.W. An object-oriented scripting interface to a legacy electronic structure code. *Comput. Sci. Eng.* **2002**; 4, 56–66.
